# Supplementary material for: Assessing Students' Understanding of Uncertainty in Undergraduate Physics Laboratory Courses at a Major Canadian University
Source: arXiv:2412.15382 source file (2025-04-29)
Supplement: Supplementary file 1 [file appendix.tex]

\begin{table*}[]
\begin{ruledtabular}
\begin{tabular}{cccccc}
{\textbf{Class}} & {\textbf{Year}} & \textbf{Format} & \textbf{Month} & \textbf{Total} & \textbf{Tested} \\
\hline
PHYS 131 & Fall 2019 & In person            & September         & 177 & 167 \\
PHYS 131 & Fall 2019 & In person            & Nov-Dec & 323 & 313 \\
PHYS 101 & Fall 2020 & Online               & September         & 475 & 452 \\
PHYS 101 & Fall 2020 & Online               & September         & 335 & 12  \\
PHYS 131 & Fall 2020 & Online               & December          & 191 & 186 \\
PHYS 101 & Fall 2021 & In person and online & September         & 77  & 34  \\
PHYS 131 & Fall 2021 & In person and online & September         & 78  & 37  \\
PHYS 101 & Fall 2022 & In person            & Sept-Oct & 82  & 22  \\
PHYS 131 & Fall 2022 & In person            & Sept-Octo & 52  & 32 
\end{tabular}
\end{ruledtabular}
\end{table*}
